# Supplementary material for: Optimizer Amalgamation
Source: arXiv:2203.06474 source file (2022-03-15)
Supplement: Supplementary file 1 [file initialization.tex]

\subsection{Initialization with Amalgamation}
\label{appendix:large-tests}
